# Supplementary material for: DiaMond: Dementia Diagnosis with Multi-Modal Vision Transformers Using MRI and PET
Source: arXiv:2410.23219 source file (2024-10-30)
Supplement: Supplementary file 1 [file supplementary.tex]

\appendix

% If you wish to avoid re-using reference numbers from the main paper,
% please uncomment the following and change the counter for `enumiv' to
% the number of references you have in the main paper (here, 6).
\let\oldthebibliography=\thebibliography
\let\oldendthebibliography=\endthebibliography

\section{Supplementary Material}
\label{supp:dataset}

\setcounter{table}{0}

\setcounter{figure}{0}

\subsection{Data Preprocessing and Splitting}
The data acquired from the ADNI dataset included all subjects from ADNI 1, ADNI 2, ADNI 3, ADNI GO that have paired MRI and FDG-PET. Data has been through pre-processing steps as shown at the ADNI website for FDG-PET\footnote{https://adni.loni.usc.edu/methods/pet-analysis-method/pet-analysis/} and for MRI\footnote{https://adni.loni.usc.edu/methods/mri-tool/mri-analysis/}. FDG-PET scans were additionally processed using SPM12\footnote{https://www.fil.ion.ucl.ac.uk/spm/software/spm12/} and CAT12\footnote{https://neuro-jena.github.io/cat12-help/}: first, the origin of all images was set to the anterior commissure region which is required for the normalization function in SPM; secondly, the scans are normalized to the MNI space using a 4-th degree B-spline interpolation; thirdly, the normalized images were registered to the MNI152 template with a voxel size of $1.5 mm^3$. In the end, all MRI scans are registered to the corresponding PET scans.  MRI scans were additionally processed using the CAT12 toolbox with the standard VBM pipeline, consisting the initial and the refined voxel-based processing. The initial pipeline applies a denoising filter, followed by internal resampling. The data is then bias-corrected, affine-registered and lastly followed by the standard SPM unified segmentation. In the second stage, skull-stripping is performed and the brain is parcellated before the final AMAP segmentation step. Finally, the tissue segments are spatially normalized to a common reference space using Geodesic Shooting. ~\cref{fig:data_preprocess} concludes the whole data preprocessing procedure. \\

\begin{figure*}[t]
    \centering
    \includegraphics[width=\linewidth]{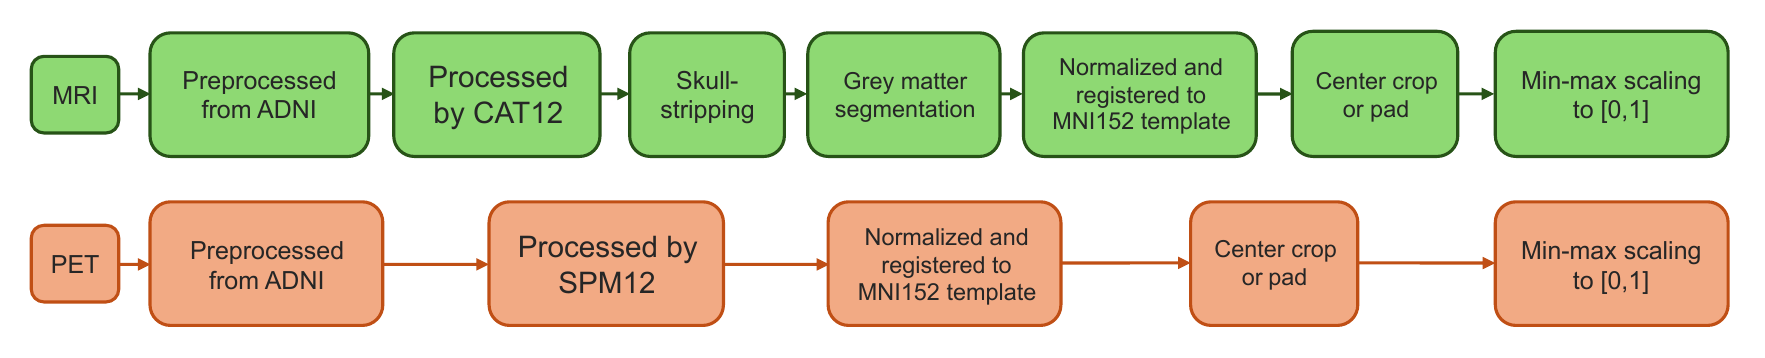}
    \caption{Dataset preprocessing of MRI and PET data.}
    \label{fig:data_preprocess}
\end{figure*}

To evenly distribute age, gender, and diagnosis across training, validation, and test data splits, we adapt the data split method from ClinicaDL~\cite{clinicadl}. First, we assess the balance of each split by computing the propensity score, which represents the probability of a sample being in the training set based on a logistic regression model that includes the known confounders~\cite{barnes2010, stern2020}. We then compare the percentiles of the propensity score distribution across the training, validation, and test sets, using the maximum deviation across all percentiles as a measure of imbalance~\cite{ho2007matching}. This process is repeated for 1000 randomly selected partitions and the partition with the minimum imbalance is finally selected.

% \begin{table}[h]
% \centering
% \scriptsize{\setlength{\tabcolsep}{0.5em}
%     \caption{Statistics for our datasets.}
%     {\begin{tabular}{lcccc}
%     \toprule
%         Dataset & Diagnosis & \ \# Samples & \ \% Female & Age \\
%         \midrule

%         \multirow{3}{*}{ADNI}
%         & CN & 379 & 50.92 & 73.46 \interval{5.93}  \\   
%         & AD & 257 & 40.47 & 74.41 \interval{7.89}  \\
%         & MCI & 611 & 41.41 & 72.31 \interval{7.30}  \\
%         \midrule

%         \multirow{3}{*}{J-ADNI}
%         & CN & 104 & 51.66 & 68.38 \interval{5.64}  \\   
%         & AD & 78 & 57.05 & 74.03 \interval{6.53}  \\
%         & MCI & 124 & 50.21 & 73.25 \interval{5.86}  \\
%         \midrule
        
%         \multirow{3}{*}{In-House}
%         & CN & 143 & 46.85 & 64.14 \interval{9.97}  \\     
%         & AD & 110 & 50.00 & 67.25 \interval{8.37}  \\
%         & FTD & 57 & 38.60 & 65.25 \interval{9.66}  \\
%     \bottomrule
%     \end{tabular}}
%     \label{tab:dataset_statistics}
%     }
% \end{table}

\subsection{Model Parameters}

\cref{tab:supple_hyperparameters} presents detailed information on the parameters used in our model and training procedure. We use the AdamW optimizer with a learning rate of $5 \times 10^{-4}$, a weight decay of $1 \times 10^{-5}$, a dropout rate of 0.0, a batch size of $16$, and cosine annealing as the learning rate scheduler. The models are trained on one NVIDIA A100 GPU with 40 GByte memory for 3,800 iterations, with early-stop to prevent overfitting. The ViT-based backbone of \modelName\ adopts a patch size of 8, a model depth of 4, a feature embedding dimension of 512, 8 attention heads, $\tau$ of 0.01. In total, the model includes $30M$ parameters.

\begin{table}[ht]
    \centering
    \caption{Parameters for \modelName.}
    \begin{tabular}{llc} \toprule
        &Parameter & Value \\\midrule
        \multirow{5}{*}{Model}   
        &Patch size & 8 \\
        &Depth & 4 \\
        &Embedding dim. & 512 \\
        &Attention heads & 8 \\
        &Model size & 30M \\       
        &$\tau$ & 0.01 \\
        \midrule
        \multirow{8}{*}{Training}
        &Batch size & 16 \\   
        &Optimizer & AdamW \\
        &Scheduler & Cosine Annealing \\
        &Learning rate & $1 \times 10^{-4}$\\
        &Weight Decay & $1 \times 10^{-5}$ \\
        &Dropout & 0.0 \\
        &Training Iterations & 3.8K \\
        &Hardware & one NVIDIA A100 GPU \\   
        \bottomrule
    \end{tabular}  
    \label{tab:supple_hyperparameters}
\end{table}

\subsection{Training Strategies}

We conducted an additional ablation study on different training strategies for DiaMond. \modelName's three independent branches allow us to initialize individual modality-specific branches with pretrained weights, potentially leveraging prior knowledge. During the training process, we explore two distinct strategies: (1) keeping the pretrained branches static (frozen) to preserve the learned representations, and (2) allowing the branches to continue learning and adapt further (continual learning). We compare these approaches to training the model entirely from scratch using 5-fold cross-validation on the ADNI dataset, specifically focusing on the classification task between CN and AD. The results indicate that incorporating pretrained models provides no substantial advantage over training the model from scratch. This suggests that the model is able to learn the relevant representations adequately through training alone. 

\begin{table}[h!]
\centering
\scriptsize
\vspace{-0.2cm}
\caption{Ablation on different training strategies.}
\vspace{-0.2cm}
{\setlength{\tabcolsep}{1em}
\label{tab:training_strategy}
\begin{tabular}{l ccc }
\toprule
Training strategy & Frozen & Continual Learning & From Scratch \\
\midrule
BACC (\%) & 91.62 \interval{2.67} & 92.36 \interval{2.41} & 92.42 \interval{2.63} \\
AUC (\%) & 96.50 \interval{1.73} & 97.17 \interval{1.25} & 97.11 \interval{1.47} \\
\bottomrule
\end{tabular}}
\end{table}
\vspace{-0.2cm}

\subsection{Differential Diagnosis of Dementia with FreeSurfer Features}

Ma et al.~\cite{ma2020differential_complete} uses whole-brain cortical thickness and volume features derived from FreeSurfer~\cite{fischl1999cortical} in a multi-scale deep neural network (MDNN) for the differential diagnosis of dementia. We further incorporate this method as a benchmark for the differential diagnosis between CN, AD, and FTD. This shape-based method achieves a balanced accuracy of 71.41\%, yet it remains lower than the performance of DiaMond.

\begin{table}[t]
\scriptsize
\caption{Differential diagnosis between CN, AD, and FTD on the in-house multi-dementia dataset.}
\label{tab:ad-ftd-main}
\begin{center}
{\setlength{\tabcolsep}{0.8em}
\begin{tabular}{lcc cc }
\toprule
% \multirow{2}{*}{Data} 
 \multirow{2}{*}{Method} &  \multicolumn{4}{c}{CN vs. AD vs. FTD} \\\cmidrule{2-5}
& BACC & F1-Score & Precision & Recall \\
\midrule
MDNN~\cite{ma2020differential_complete} & 71.41 \interval{2.24} & 71.99 \interval{2.12} & 73.24 \interval{1.77} & 73.50 \interval{2.02} \\
\modelName & \textbf{76.46 \interval{3.33}} & \textbf{75.53 \interval{4.38}}  & \textbf{76.76 \interval{4.88}} & \textbf{75.39 \interval{3.23}}  \\
\bottomrule
\end{tabular}}
\end{center}
\end{table}
